# Supplementary material for: Mixture of Robust Experts (MoRE):A Robust Denoising Method towards multiple perturbations
Source: arXiv:2104.10586 source file (2025-03-26)
Supplement: Supplementary file 1 [file appendix.tex]

\setcounter{section}{0}
\setcounter{figure}{0}
\setcounter{equation}{0}
\makeatletter 
\renewcommand{\thefigure}{A\@arabic\c@figure}
\makeatother
\setcounter{table}{0}

\appendix
\onecolumn
\section*{Appendix}

\section{Hyperparameter Setting}
\label{hyper-para}
%This section give some definitions about the hyperparameter used in this paper. $\epsilon$ is the bounded size of $\ell_p$ attacks. t and light is two hyperparameters that help us to simulate the Fog. Specifially, t is the factor to indicate how thick the fog that we want to simulate. Light is the factor to indicate the atmospheric light of the Fog used in this paper. Bright is the factor to form the snow. This hyperparameter helps us to know how bright to make our snow.
% rephrase first paragraph
\paragraph{}

 This section provides details on the hyperparameters used in this paper. All single experts and gating module are based on the ResNet18. In adversarially training phase, the adversarial examples are simulated by using Projected Gradient Descent (PGD) method and are also based on ResNet18. Here $\epsilon$ denotes the bound on $\ell_p$ PGD attacks. The notation $p$ indicates two different norms, which are $\ell_2$ and $\ell_\infty$ norm. For the 
specific value, in CIFAR-10, for $\ell_2$ perturbations, $\epsilon$ are $0.5$ and $1.0$. For $\ell_\infty$ perturbations, $\epsilon$ are $\frac{6.0}{255}$ and $\frac{8.0}{255}$. 
 The number of PGD attack steps is $20$, and the perturbation step size is $\frac{epsilon}{5}$ for $\ell_2$ and $0.01$ for $\ell_\infty$.
 
 For two natural perturbations, fog and snow ,used in this paper,  there are also having different hyperparemeters to simulate these perturbations. 
 In fog, we use \emph{t} and \emph{light} as two hyperparameters, where \emph{t} is the factor to control the thickness of the fog and \emph{light} is the factor to control the atmospheric lightness of the fog. For natural perturbations of snow, we use \emph{bright} as a hyperparameter, which controls the brightness of the snow. In section B of the appendix, \textbf{fog1} is specified with $\emph{t}=0.15$ and $\emph{light}=0.6$, whereas \textbf{fog2} is specified with $\emph{t}=0.12$ and $\emph{light}=0.8$; \textbf{snow1} is specified with $\emph{brightness}=2.5$, whereas \textbf{snow2} is specified with $\emph{brightness}=2.0$. 

For the training processes of clean experts, different adversarially trained and natural perturbations robustly trained experts, we use SGD optimizer with the learning rate ($lr$) updating scheduler that decreases the learning rate along with the increment of the number of epochs. We use initial $lr=0.1$ and  
use $0.005$ to update the initial $lr$. For the training process of our {\em MoRE} structure, we also use SGD optimizer with a similar $lr$ updating scheduler. The $lr$ updating scheduler strategy is adopted from the baseline code~\cite{maini2019adversarial}, which could improve the training efficiency and accuracy.

For testing the robustness of our system under adaptive attack (Section~\ref{sec:adaptive}), we adopt our mixing trained {\em MoRE} structure, including S1 and S2, as the based model to generate adaptive adversarial examples. About the detailed parameter values, such as $\epsilon$ bound, attack steps number and step size, of adaptive attack are all mentioned before.
% in CIFAR-10, for $\ell_2$ perturbations, $\epsilon$ are $\frac{20}{255}$ and $\frac{40}{255}$. For $\ell_\infty$ perturbations, $\epsilon$ are $\frac{2.0}{255}$ and $\frac{4.0}{255}$. In Tiny-ImageNet, for $\ell_2$ perturbations, $\epsilon$ are $\frac{40}{255}$ and $\frac{60}{255}$. For $\ell_\infty$ perturbations, $\epsilon$ are $\frac{4.0}{255}$ and $\frac{6.0}{255}$.

About baseline comparisons, we train all models (Max, Averahe and MSD) with 30 epochs, batch size 128, and cross entropy as our training loss function. All baseline experiments also have the same experimential setting as our {\em MoRE} mixing process and are performed on CIFAR-10. Additionally, all of these
%use Adam~\cite{KingmaB2015adam} as our optimiz
 comparing baselines use SGD with the similar $lr$ update scheduler. And the parameter values of each process in both datasets are just same as the values used in above mentioned {\em MoRE} generating process.
%
% Code for all our experiments are at \textcolor{blue}{\url{https://github.com/ChaduCheng/Mixture-of-Robust-Experts-MoRE-} }
%For training all PGD and MSD attacks models and generating all PGD and MSD attack images, we uses 10 attack steps. In each attack step, we set the step size to $\frac{2.0}{255}$.   

\section{Additional Experimental Results}

In Tables~\ref{indiv_baseline_cifar10}, we report the confusion matrix of the test accuracy of different experts for CIFAR-10, respectively. 

% In Tables~\ref{table:moe_adv} and~\ref{table:MOE_nature}, we present the performance of our proposed structure 1 and 2 when encountering adversarial examples and natural perturbations in CIFAR-10. Similar results for Tiny-ImageNet 
% could be found in Table~\ref{table:moe_nat_timage} and~\ref{table:moe_adv_timage}. Finally, we show the quantitative results for our proposed S2-MoRE method compared with rest of the baselines on CIFAR-10 and Tiny-ImageNet in Table~\ref{table:compare_baseline_cifar} and~\ref{table:compare_baseline_timage}.

\begin{table*}[htb]
\centering
%\renewcommand\thetable{\alph{table}}
%\small{
 \caption{The test accuracy (\%) of each clean, adversarial trained and natural perturbations trained individual model (or expert) for CIFAR-10 dataset. 
  } 
\label{indiv_baseline_cifar10}
  \vspace{2mm}
 \adjustbox{max width=2.5\textwidth}{
\begin{tabular}{l|llllllllll}
\toprule
% \multicolumn{1}{c}{weights\textbackslash image} &
\multicolumn{1}{c}{types} &
  clean  &
  \begin{tabular}[c]{@{}l@{}}$\ell_2$  ($\epsilon$ =\\ 0.5)\end{tabular} &
  \begin{tabular}[c]{@{}l@{}}$\ell_2$  ($\epsilon$ =\\ 1.0)\end{tabular} &
  \begin{tabular}[c]{@{}l@{}}$\ell_\infty$ ($\epsilon$ = \\ 6/255)\end{tabular} &
  \begin{tabular}[c]{@{}l@{}}$\ell_\infty$  ($\epsilon$ = \\ 8/255)\end{tabular} &
   \begin{tabular}[c]{@{}l@{}}fog1\end{tabular} &
  \begin{tabular}[c]{@{}l@{}}fog2\end{tabular} &
  \begin{tabular}[c]{@{}l@{}}snow1 \end{tabular} &
  \begin{tabular}[c]{@{}l@{}}snow2\end{tabular}  &
  Average \\ \hline
clean   &
  93.70 &
  &
   &
  &
   &
   &
   &
   &
   &
  
  \\ \hline
\begin{tabular}[c]{@{}l@{}}$\ell_2$ ($\epsilon$ =\\ 0.5)\end{tabular} &
  86.99 &
  69.57 &
  &
  &
  &
  &
  &
  &
  &
  
  \\ \hline
\begin{tabular}[c]{@{}l@{}}$\ell_2$  ($\epsilon$ =\\ 1.0)\end{tabular} &
   80.73&
   &
   48.91&
   &
   &
   &
   &
   &
   &
   
  \\ \hline 
\begin{tabular}[c]{@{}l@{}}$\ell_\infty$ ($\epsilon$ =\\ 6/255)\end{tabular}     &
   85.07&
   &
   &
   56.73&
   &
   &
   &
   &
   &
   
 \\ \hline
\begin{tabular}[c]{@{}l@{}}$\ell_\infty$ ($\epsilon$ =\\ 8/255)\end{tabular}    &
   81.28&
   &
   &
   &
   48.01&
   &
   &
   &
   &
   
 \\ \hline
\begin{tabular}[c]{@{}l@{}}fog1\end{tabular} &
  54.3 &
  &
  &
  &
  &
  79.76&
  &
  &
  &
  
  \\ \hline
\begin{tabular}[c]{@{}l@{}}fog2\end{tabular} &
  67.26 &
   &
   &
   &
   &
   &
  81.52 &
   &
   &
  
  \\ \hline 
\begin{tabular}[c]{@{}l@{}}snow1\end{tabular} &
  80.84 &
   &
   &
   &
   &
   &
   &
   75.23&
   &
  
 \\ \hline
\begin{tabular}[c]{@{}l@{}}snow2\end{tabular} &
  82.34 &
  &
  &
  &
  &
  &
  &
  &
  76.65 &
  
  \\ \bottomrule  
\end{tabular}
}
\end{table*}

\begin{table*}[ht!]
%\small{
\centering
 \caption{Test accuracy on perturbations specific to an individual expert on CIFAR-10.
  } 
\label{table:indiv_baseline_cifar10_simple}
\vspace{2mm}
%  \adjustbox{max width=1\textwidth}{
\begin{tabular}{l|l|llll|llll}
\toprule
% \multicolumn{1}{c}{weights\textbackslash image} &
\multicolumn{1}{c|}{Models} &
  clean  &
  \begin{tabular}[c]{@{}l@{}}$\ell_2$  ($\epsilon$ =\\ 0.5)\end{tabular} &
  \begin{tabular}[c]{@{}l@{}}$\ell_2$  ($\epsilon$ =\\ 1.0)\end{tabular} &
  \begin{tabular}[c]{@{}l@{}}$\ell_\infty$ ($\epsilon$ = \\ 6/255)\end{tabular} &
  \begin{tabular}[c]{@{}l@{}}$\ell_\infty$  ($\epsilon$ = \\ 8/255)\end{tabular} &
  \begin{tabular}[c]{@{}l@{}}fog1\end{tabular} &
  \begin{tabular}[c]{@{}l@{}}fog2\end{tabular} &
  \begin{tabular}[c]{@{}l@{}}snow1\end{tabular} &
  \begin{tabular}[c]{@{}l@{}}snow2\end{tabular} 
   \\ \hline
  Single Experts  &
  93.7 &
  69.57 &
  50.49 &
  55.4 &
  48.73 &
  79.76 &
  81.52 &
  75.23 &
  76.65 
  \\ \bottomrule  
\end{tabular}
% }
\end{table*}
\begin{table*}[ht!]
\centering
 \caption{Test accuracy (\%) of {\em MoRE} under different perturbations in CIFAR-10.
  } 
  \label{MoE_results_cifar}
  \vspace{2mm}
\begin{tabular}{l|llllllllll}
\toprule
\multicolumn{1}{c|}{Types} &
  clean  &
  \begin{tabular}[c]{@{}l@{}}$\ell_2$  ($\epsilon$ =\\ 0.5)\end{tabular} &
  \begin{tabular}[c]{@{}l@{}}$\ell_2$  ($\epsilon$ =\\ 1.0)\end{tabular} &
  \begin{tabular}[c]{@{}l@{}}$\ell_\infty$ ($\epsilon$ =\\ 6/255)\end{tabular} &
  \begin{tabular}[c]{@{}l@{}}$\ell_\infty$  ($\epsilon$ =\\ 8/255)\end{tabular} &
  \begin{tabular}[c]{@{}l@{}}fog1\end{tabular} &
  \begin{tabular}[c]{@{}l@{}}fog2\end{tabular} &
  \begin{tabular}[c]{@{}l@{}}snow1\end{tabular} &
  \begin{tabular}[c]{@{}l@{}}snow2\end{tabular} &
  Average \\ \hline
  {\em adv MoRE}&
  74.43 &
  62.16 &
  48.75 &
  47.73 &
  38.54 &
   - &
   - &
   - &
   - &
  54.26 \\ 
  \begin{tabular}[c]{@{}l@{}}{\em nat MoRE}\end{tabular} &
  90.01 &
   - &
   - &
   - &
   - &
  87.25 &
  88.16 &
  86.27 &
  83.62 &
  87.06
  \\
  \begin{tabular}[c]{@{}l@{}}{\em all MoRE}\end{tabular} &
  75.66 &
  62.74&
  46.83 &
  50.51 &
  40.86 &
  49.98 &
  54.78 &
  61.07 &
  52.07 &
  55.02
  \\ \bottomrule
\end{tabular}
\end{table*}

\section{Details of Ablation Study}
In this section we give a detailed weights distribution of the first layer of our Hierarchically Gated {\em MoRE} (S2).
%In this section, we would describe the detailed processes about this thought by adding some more comprehensive experimental results. 

% Tables~\ref{Weight_all_exp_cifar} show the specific distributions of weight values when using different types of inputs for training on CIFAR-10. 
% In these two tables, the weights for a specific expert are larger than other experts' with corresponding types of input data for training. We name this characteristic as dynamic weight value distribution.
% For example, in Table~\ref{Weight_all_exp_cifar}, we know that the weight of the $\ell_2$ expert ($0.2929+0.3697$) is obviously the highest value among different trained experts. For natural perturbations, specifically, weights of fog($0.4060+0.3936$) is also highest.  

Additionally, as mentioned in the major part, our S1 {\em MoRE} has a notable shortcoming, the performance of mixing all types of trained experts together is not so good, comparing with just solely mixing clean trained experts with adversarially trained or naturally robutslly trained experts.. For instance, when mixing all clean expert, $\ell_2$ as well as $\ell_\infty$ adversarial experts, fog and snow experts together, the classifying accuracy of each type of expert is worse than another mixing situation, i.e.,  mixing $\ell_2$ and $\ell_\infty$ with different $\epsilon$ together. 
After obtaining this characteristic, we come to an inspiration, which uses this weights distribution as an basis to identify whether the testing inputs belong to which types of trained experts (clean, adversarial or natural perturbations), to overcome this shortcoming.

We also present the experimental results to quantify the performance gain of {\em MoRE} over individual experts. Our {\em MoRE} model referred in Section~\ref{more1} is tested. Our {\em MoRE} model are optimized using the training process as mentioned in Section~\ref{sec:more-train}. Our robustness performance of our different {\em MoRE} systems ({\em adv MoRE:} mixing clean experts with all adversarial trained experts; {\em all MoRE:} mixing clean experts with all adversarial trained and natural perturbation experts) on CIFAR-10 are reported in Tables~\ref{MoE_results_cifar}. These results show %that S2 is significantly more robust as compared to S1. Further, S2 {\em MoRE}
our system is able to achieve high robustness to all perturbation types compared to the most individual robust experts when defend against different perturbation types.
%even on their specific perturbation types. 
These results reinforce or hypothesis that the right combination of multiple robust experts can outperform the best individual expert in the ensemble.

Concretely, for the detailed applying process, we can feed the testing images in an image types classifying gating as the first level of our Hierarchically Gate {\em MoRE} (S2) and obtain the highest weights first. After that, the corresponding type of {\em MoRE} structure whose weighted is the dominated one could finally help us to finish this classifying task. 
Those different types of {\em MoRE} are pregenerated, and these types include clean type {\em MoRE}, adversarial type {\em MoRE} and natural perturbations types {\em MoRE}.
Since all weights are required in this image type classifying task, we use {\em Softmax Weighting gating module} as our classifier. The major purpose of this classifying task is to indicate the inputs belong to which kind of experts. Therefore, the number of the output label should be $3$, including clean, adversarial and natural perturbations type. For clean type, we could use clean expert directly. However, for adversarially trained or natural perturbation robustly trained experts, we adopt the most represented particular type ($\ell_2$ or $\ell_\infty$, fog or snow) to indicate its corresponding expert species (adversarial or natural perturbation). In this paper, we choose $\ell_2$ and fog to represent $\ell_p$ adversarial example and natural perturbation type. 
